# Supplementary material for: Stability of the personal relationship networks in a longitudinal study of middle school students
Source: arXiv:2303.03786 source file (2023-09-01)
Supplement: Supplementary file 1 [file supplementary_information.pdf]

# Supplementary Information on "Stability of the personal relationship networks in a longitudinal study of middle school students"


Diego Escribano,[1] Francisco J. Lapuente,[2,3] José A. Cuesta,[1,4], Robin I.M. Dunbar[5] and Angel Sánchez[1,4]

[1]Grupo Interdisciplinar de Sistemas Complejos (GISC), Departamento de Matemáticas, Universidad Carlos III de Madrid, 28911 Leganés, Madrid, Spain

[2]Instituto de Enseñanza Secundaria Blas de Otero, 28024 Madrid, Spain

[3]Departamento de Biología y Geología, Física y Química Inorgánica, Universidad Rey Juan Carlos, 28933, Móstoles, Madrid, Spain

[4]Instituto de Biocomputación y Física de Sistemas Complejos (BIFI), Universidad de Zaragoza, 50018 Zaragoza, Spain

[5]Department of Experimental Psychology, University of Oxford, Oxford OX2 6GG, UK


## S1 Number of responders across groups

In our research, we have students responding to our surveys during the academic years 2020-2021 and 2021-2022. To identify them uniquely, we associate each student with the course they are currently taking in the year 2021-2022. As we are only considering students that answered all five surveys, this implies that there are practically no students in 1st-year ESO, because they only participated in waves 4 and 5. Those that are still listed as being in 1st-year ESO are therefore "repetidores".

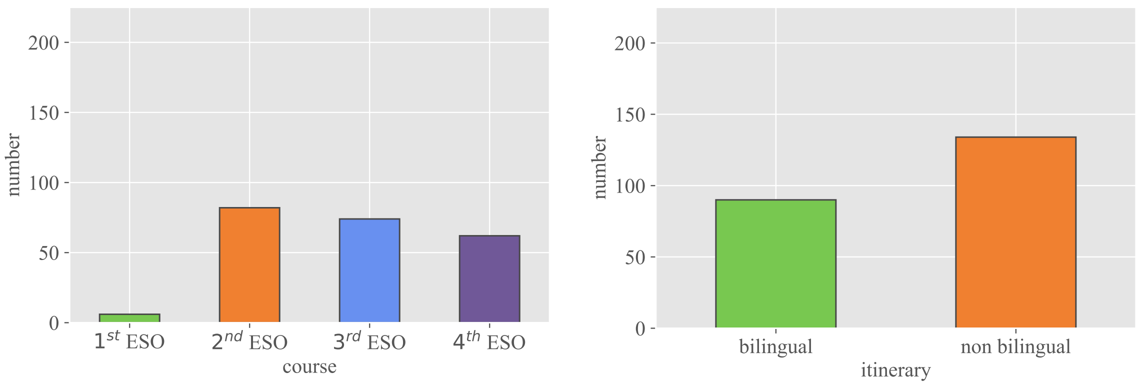


Fig. S1: **Distribution of the students participating in all five waves -** Left: by course. Right: by itinerary.

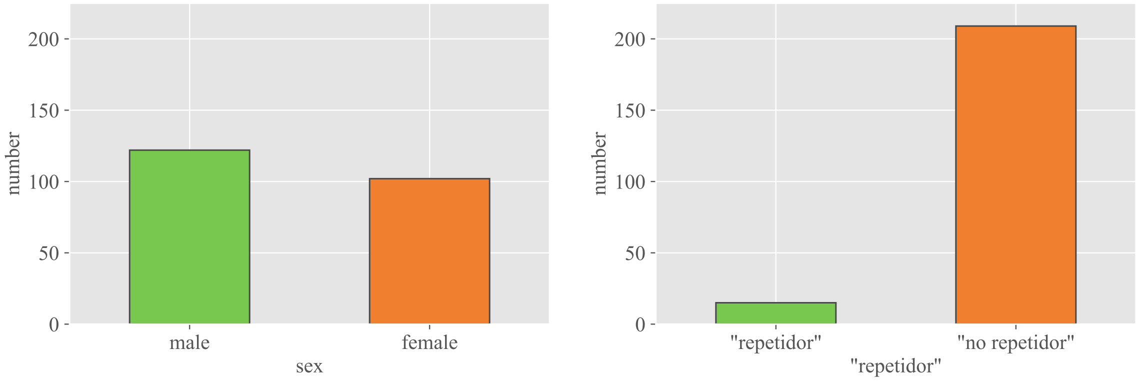


Fig. S2: **Distribution of the students participating in all five waves -** Left: by sex. Right: by "repetidores" or not.

# S2 Number of friendships

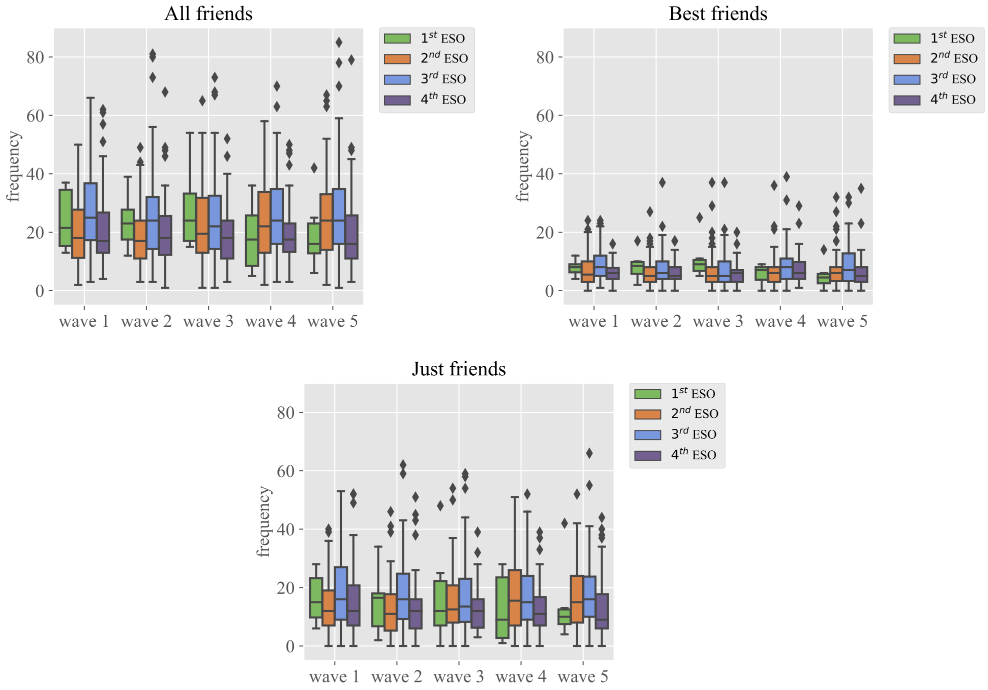


Fig. S3: **Number of friendships declared by course -** Left: all friends. Right: best friends. Bottom: just friends.

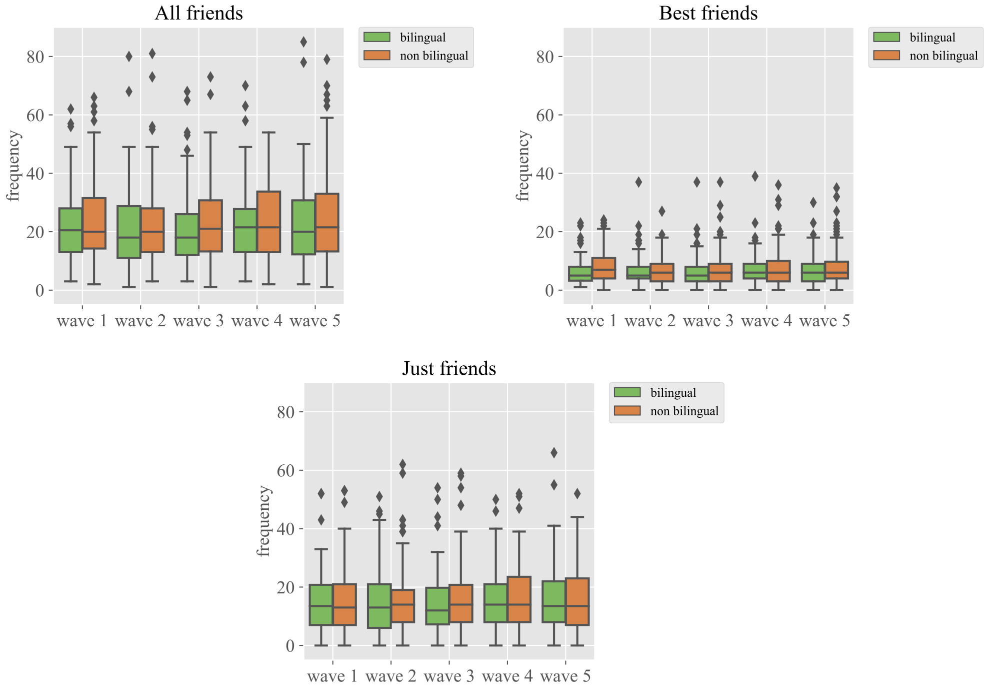


Fig. S4: **Number of friendships declared by itinerary -** Left: all friends. Right: best friends. Bottom: just friends.

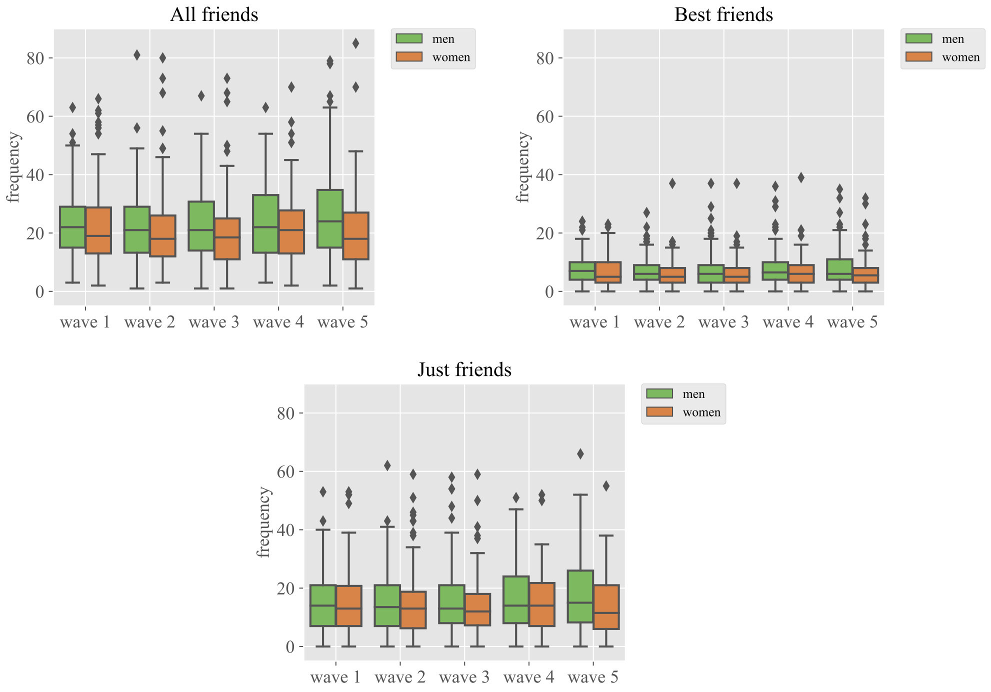


Fig. S5: **Number of friendships declared by gender -** Left: all friends. Right: best friends. Bottom: just friends.

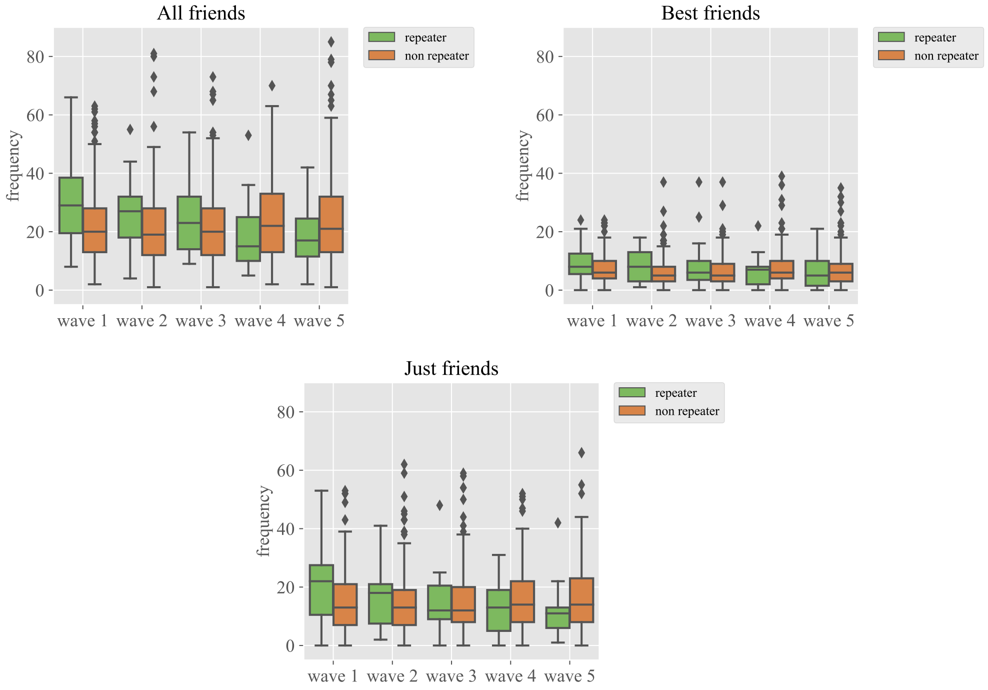


Fig. S6: **Number of friendship declared by "repetidores" or not -** Left: all friends. Right: best friends. Bottom: just friends.

# S3 $\mu$ parameter.

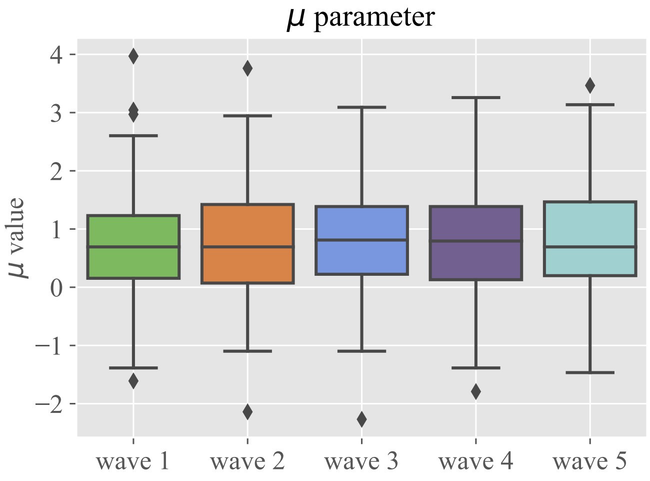


Fig. S7: $\mu$ **parameter distribution across waves**

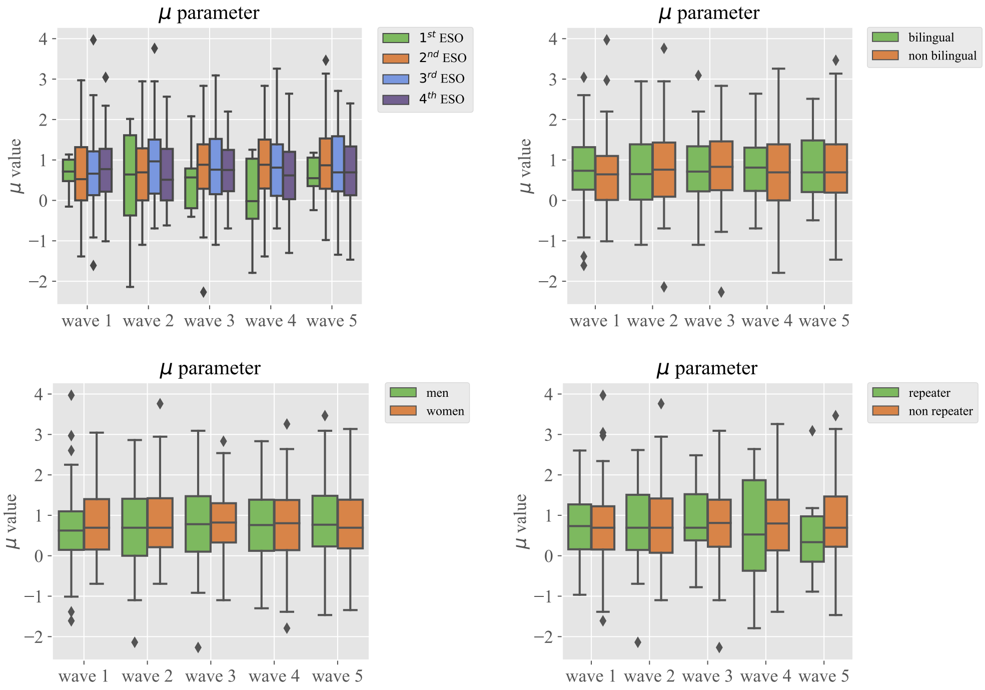


Fig. S8: $\mu$ **parameter distribution with division by groups** - Top left: by course. Top right: by itinerary. Bottom left: by gender. Bottom right: by "repetidores" or not.

# S4 Slopes of the linear fit to aggregate evolution over time

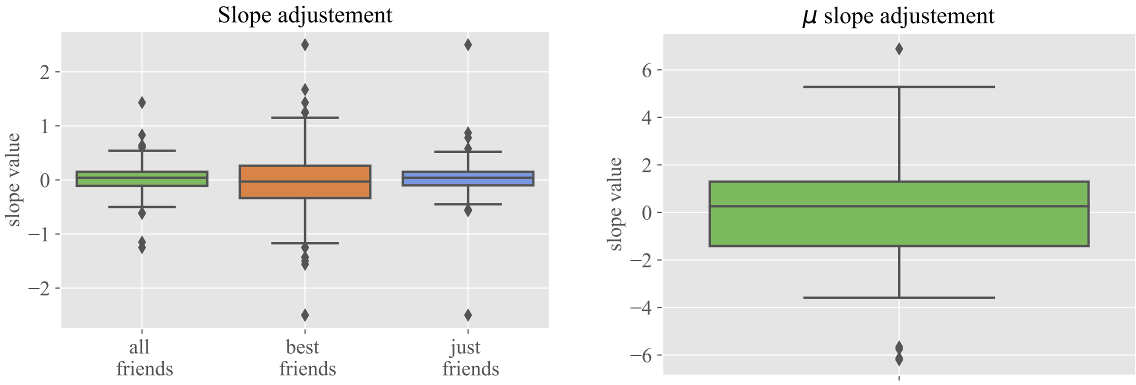


Fig. S9: **Slope of linear fits to the evolution** - Left: number of friendships. Right: $\mu$ parameter.

## S5 Transitions of relationships between waves

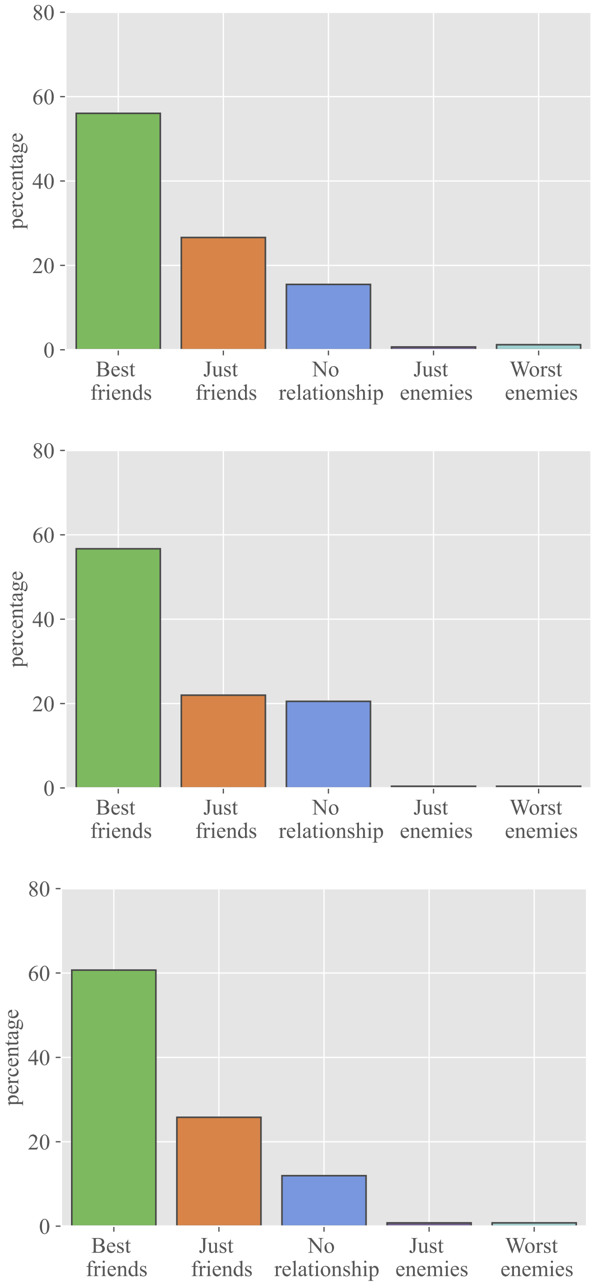


Fig. S10: **Best friends transitions -** Percentage of individuals that ended up in a given category in wave $n$, when they were marked as "best friend" in the previous wave (conditional probability $P(x, w_n| + 2, w_{n-1})$). Top: from wave 1 to wave 2. Middle: from wave 2 to wave 3. Bottom: from wave 3 to wave 4.

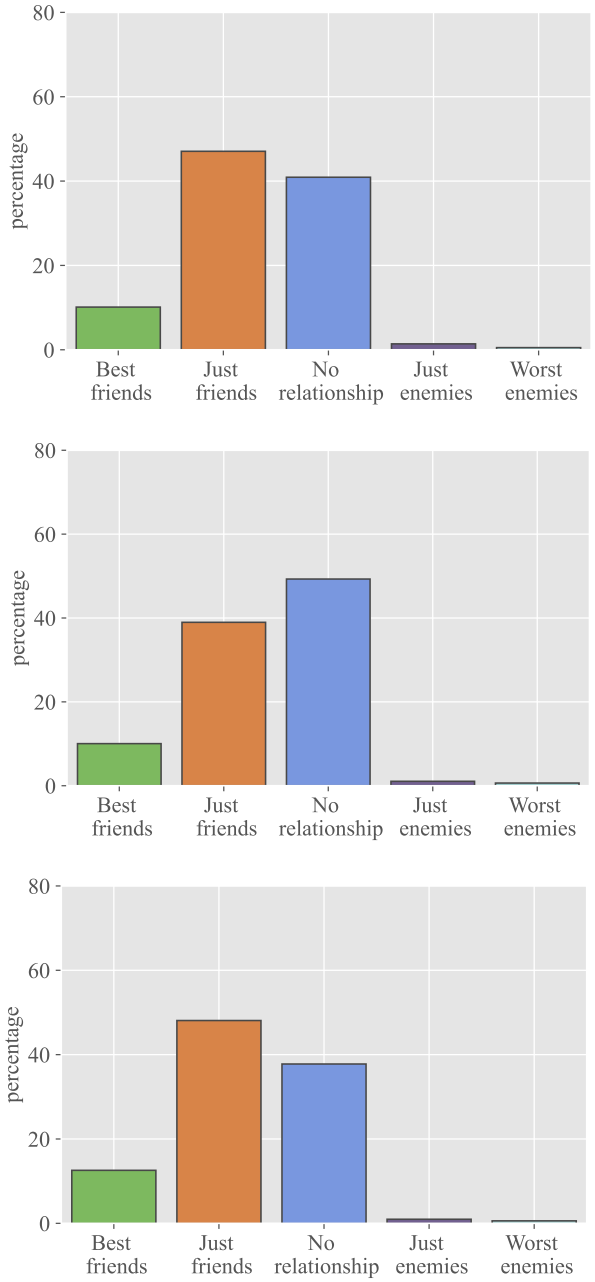


Fig. S11: **Friends transitions** - Percentage of individuals that ended up in a given category in wave $n$, when they were marked as "just friend" in the previous wave (conditional probability $P(x, w_n| + 1, w_{n-1})$). Top: from wave 1 to wave 2. Middle: from wave 2 to wave 3. Bottom: from wave 3 to wave 4.

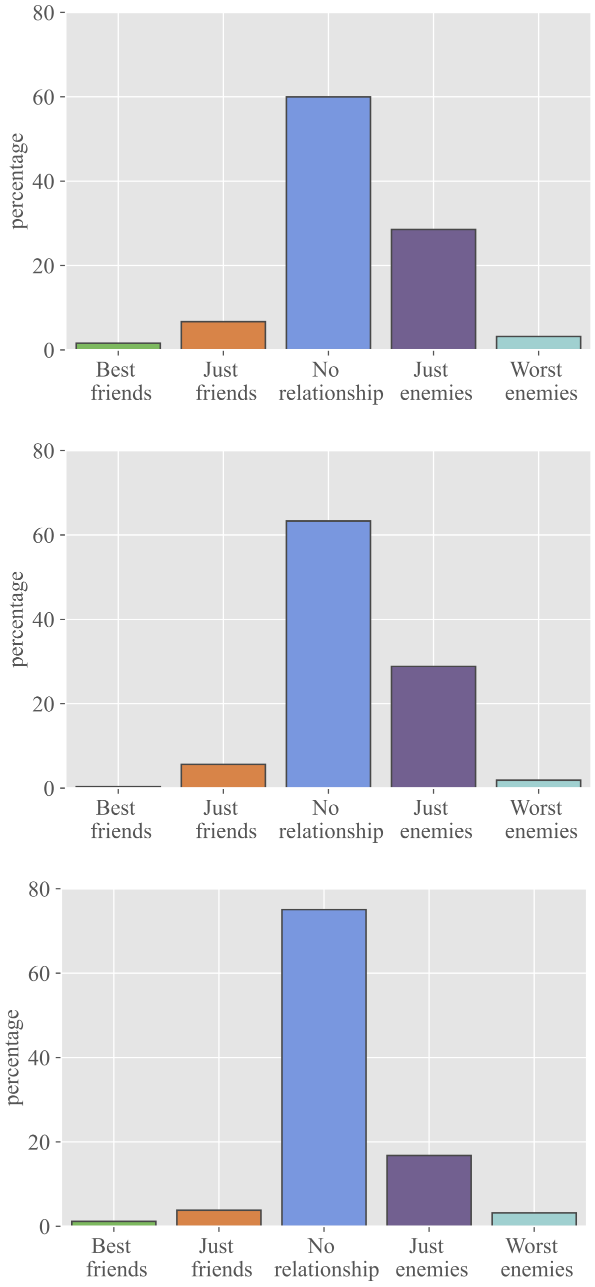


Fig. S12: **Enemies transitions -** Percentage of individuals that ended up in a given category in wave $n$, when they were marked as "just enemy" in the previous wave (conditional probability $P(x, w_n| -1, w_{n-1})$). Top: from wave 1 to wave 2. Middle: from wave 2 to wave 3. Bottom: from wave 3 to wave 4.

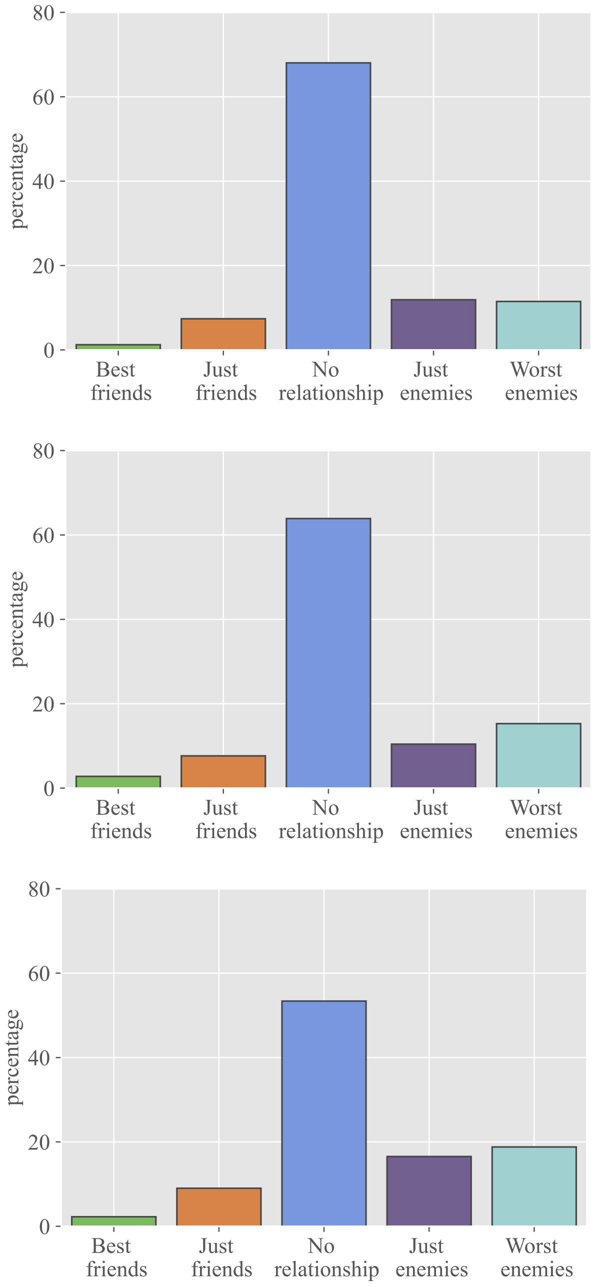


Fig. S13: **Worst enemies transitions -** Percentage of individuals that ended up in a given category in wave $n$, when they were marked as "worst enemy" in the previous wave (conditional probability $P(x, w_n| - 2, w_{n-1})$). Top: from wave 1 to wave 2. Middle: from wave 2 to wave 3. Bottom: from wave 3 to wave 4.

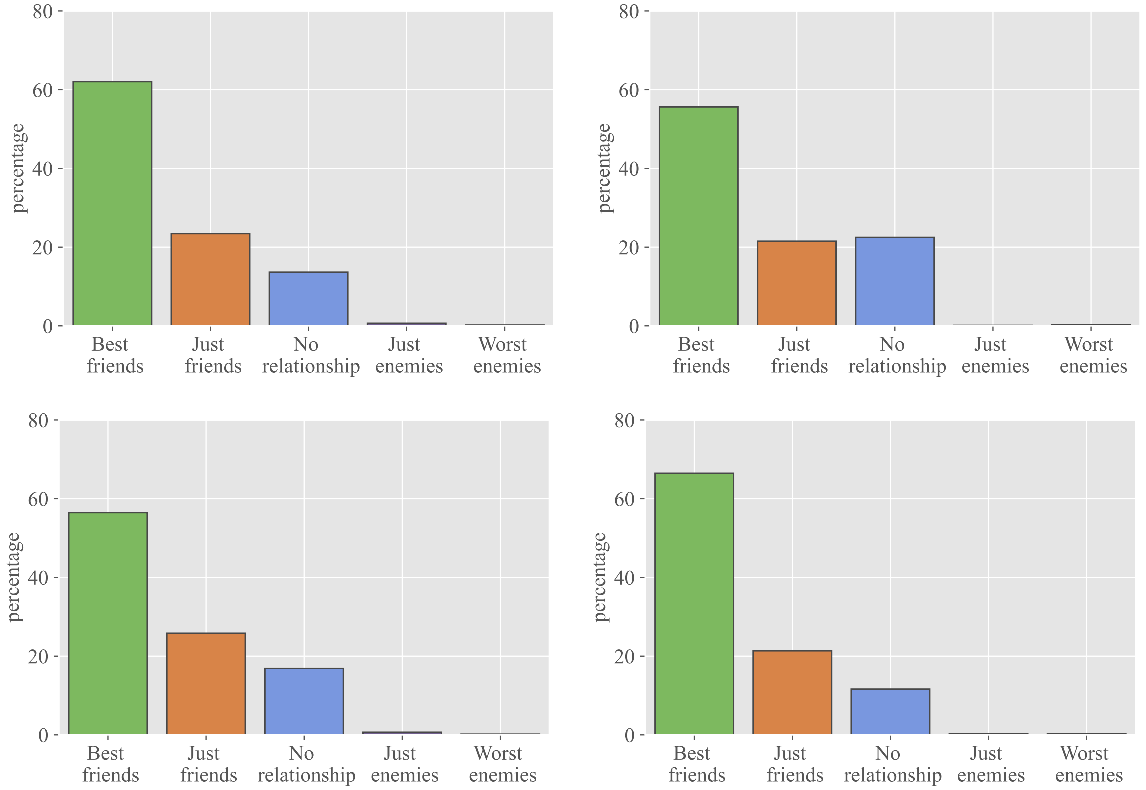


Fig. S14: **Best friends origin** - Percentage of individuals that end up as “best friends” in wave $n$ and were marked in any category in the previous wave (conditional probability $P(x, w_{n-1}|2, w_n)$). Top left: from wave 1 to wave 2. Top right: from wave 2 to wave 3. Bottom left: from wave 3 to wave 4. Bottom right: from wave 4 to wave 5.

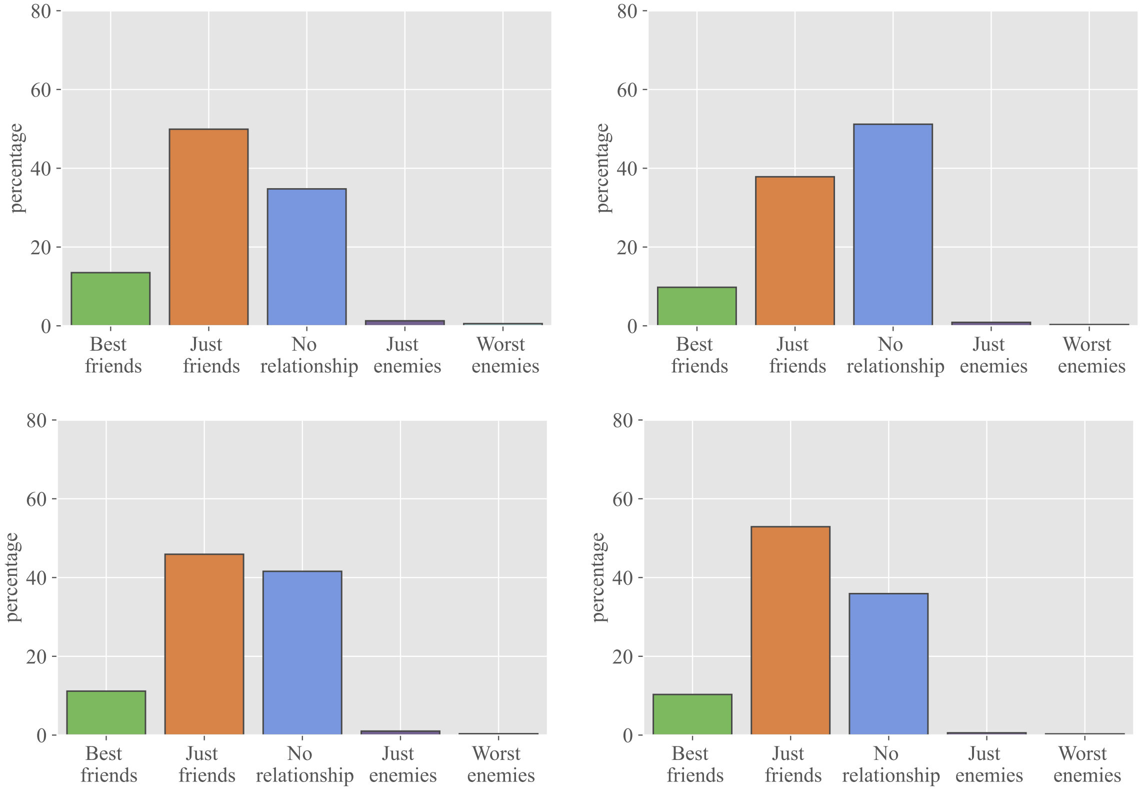


Fig. S15: **Just friends origin** - Percentage of individuals that end up as "just friends" in wave $n$ and were marked in any category in the previous wave (conditional probability $P(x, w_{n-1}|1, w_n)$). Top left: from wave 1 to wave 2. Top right: from wave 2 to wave 3. Bottom left: from wave 3 to wave 4. Bottom right: from wave 4 to wave 5.

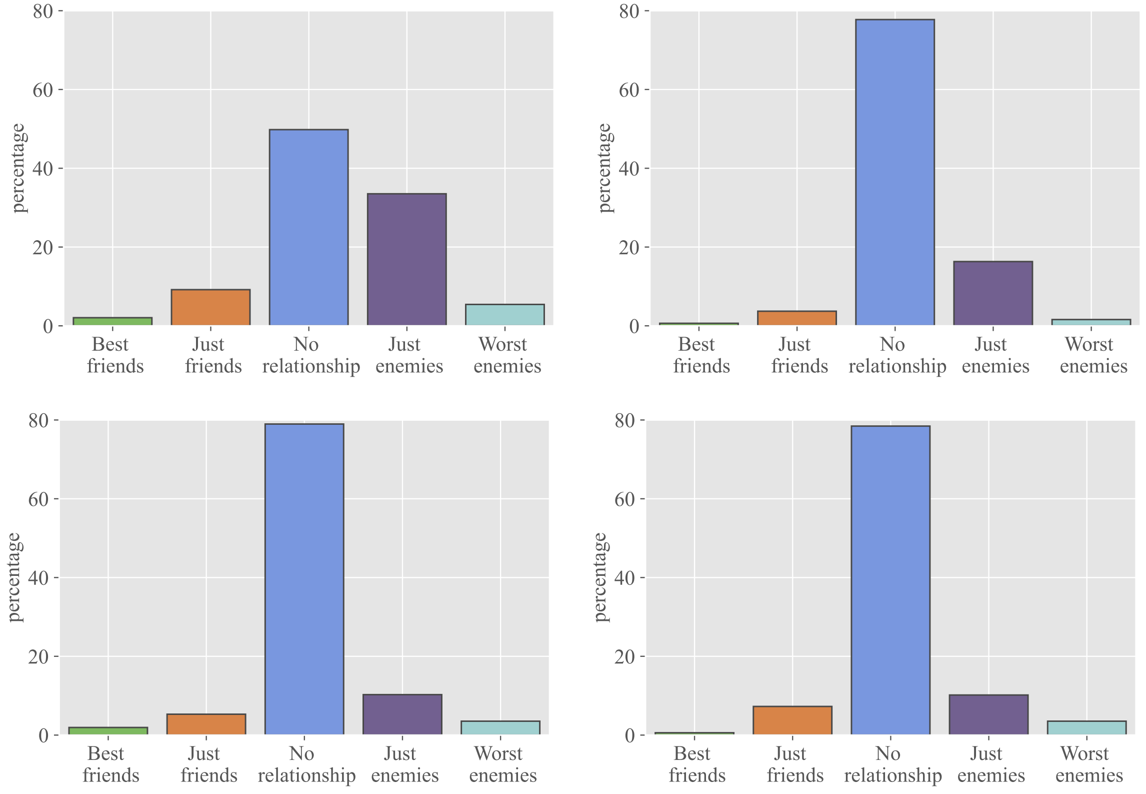


Fig. S16: **Just enemies origin** - Percentage of individuals that end up as "just enemies" in wave $n$ and were marked in any category in the previous wave (conditional probability $P(x, w_{n-1}| -1, w_n)$). Top left: from wave 1 to wave 2. Top right: from wave 2 to wave 3. Bottom left: from wave 3 to wave 4. Bottom right: from wave 4 to wave 5.

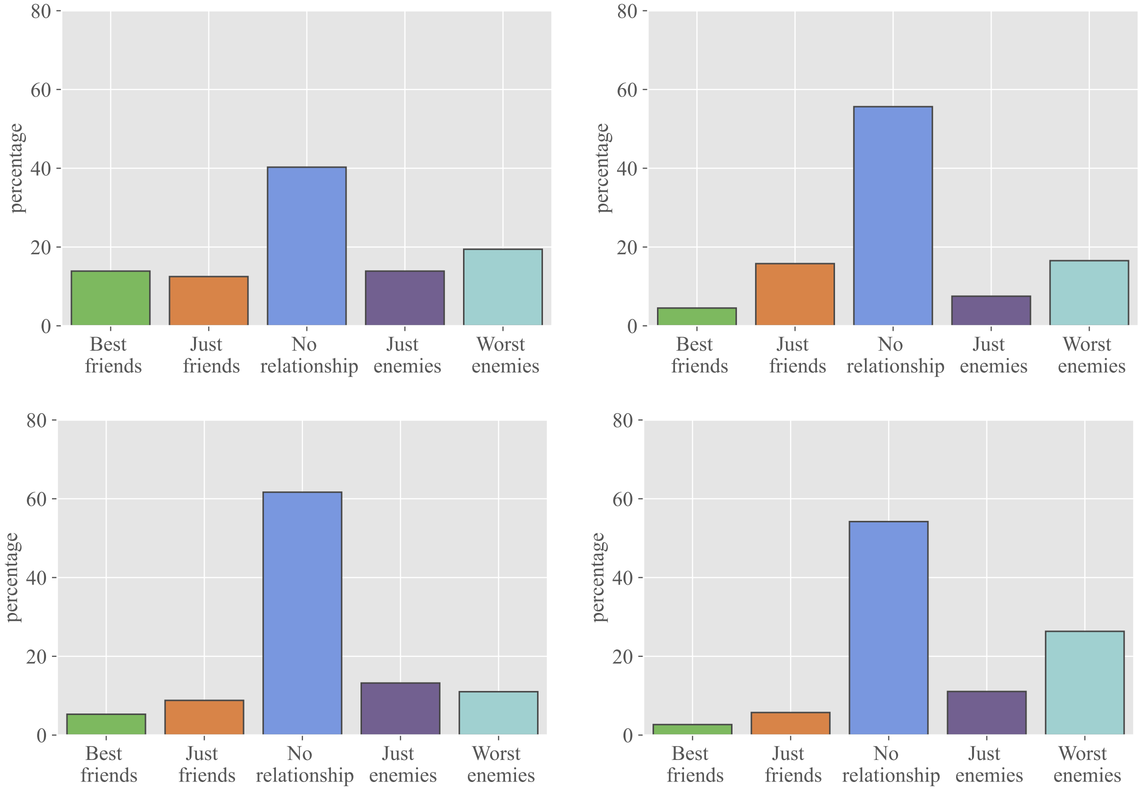


Fig. S17: **Worst enemies origin -** Percentage of individuals that end up as "worst enemies" in wave $n$ and were marked in any category in the previous wave (conditional probability $P(x, w_{n-1}|-2, w_n)$). Top left: from wave 1 to wave 2. Top right: from wave 2 to wave 3. Bottom left: from wave 3 to wave 4. Bottom right: from wave 4 to wave 5.

# S6 Number of S-S, S-D, D-S, and D-D relationships

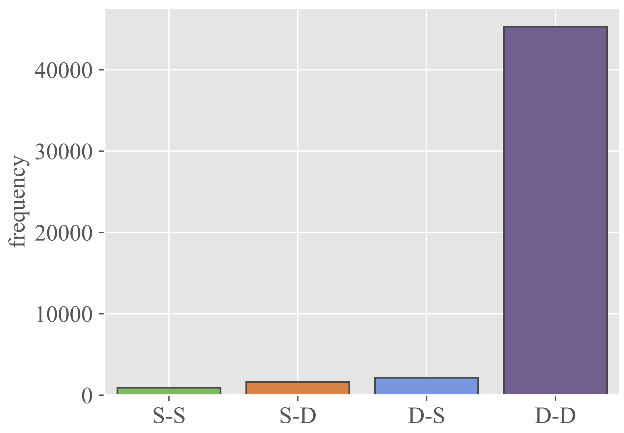


Fig. S18: **Number of pairs of relationships -** S-S: same class in both academic years. S-D: same class the first year and different the second. D-S: different class the first year and same the second. D-D: different classes in both academic years.

# S7 Reciprocity

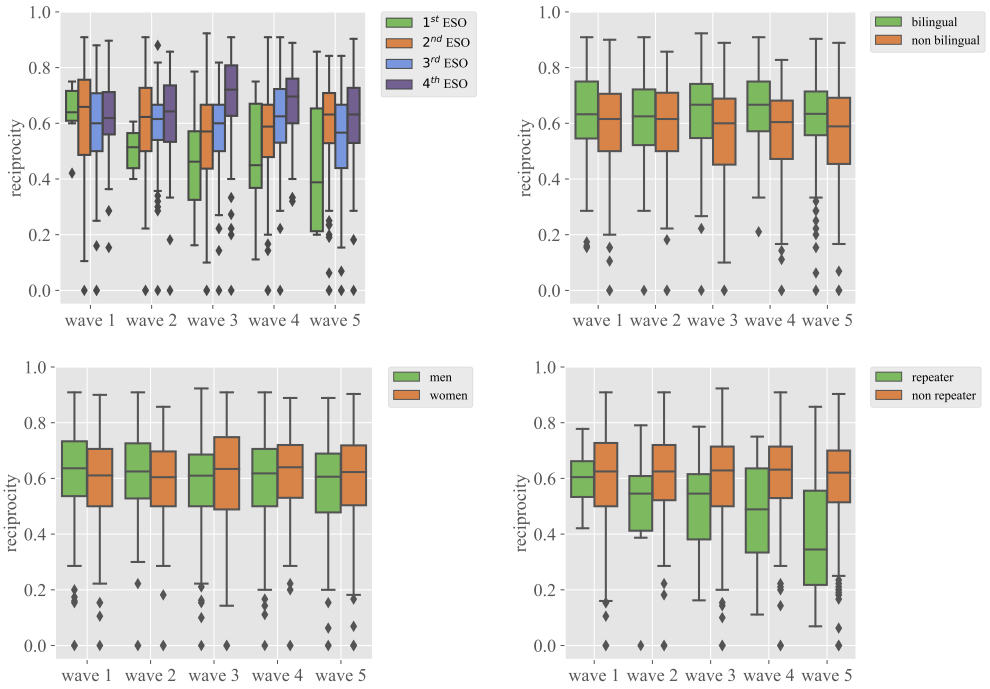


Fig. S19: **Reciprocal relationships -** Top left: by course. Top right: by itinerary. Bottom left: by gender. Bottom right: by “repetidores” or not.

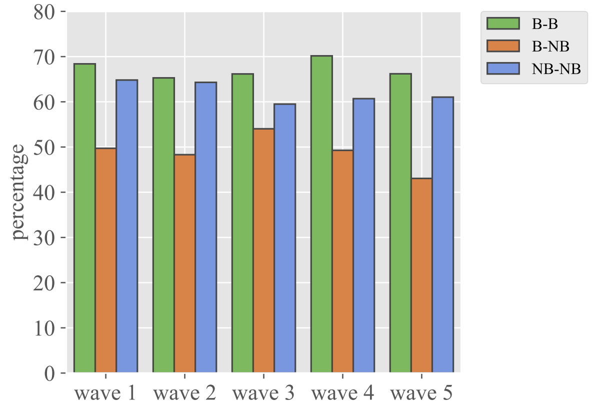


Fig. S20: **Reciprocity per itinerary** - B-B (bilingüe-bilingüe), B-NB (bilingüe-no bilingüe), NB-NB (no bilingüe-no bilingüe).

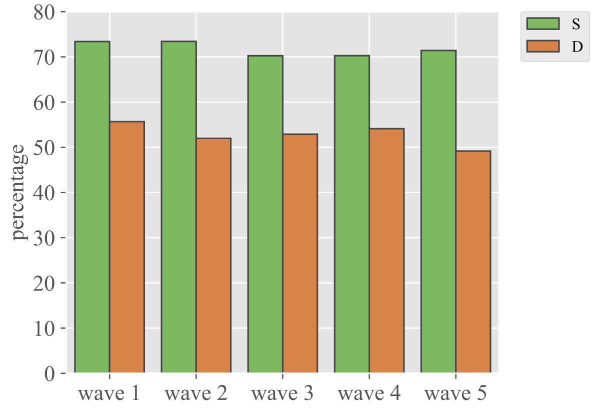


Fig. S21: **Reciprocity per group** - S (same group), D (different group).

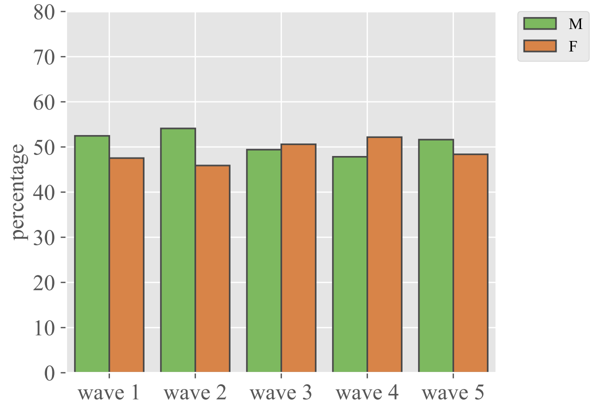


Fig. S22: **Reciprocity per sex** - Percentage of non-reciprocal relationships that are directed from men to women (green) and from women to men (orange) in each wave.

## S8 Reciprocity of negative relationships

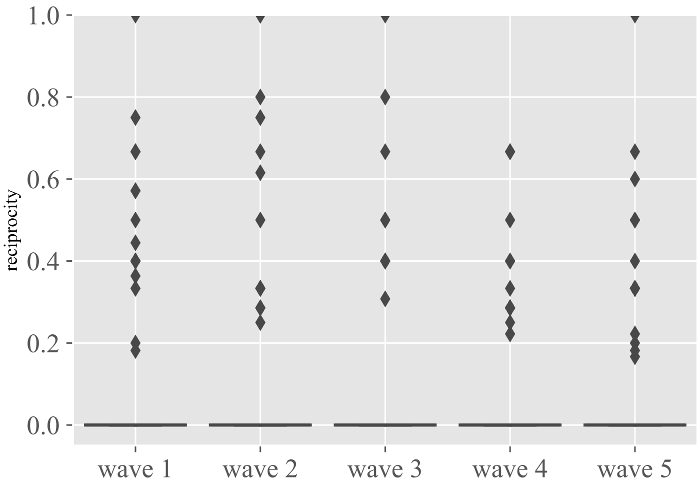


Fig. S23: **The structure of friendships** - Replica of Figure 1 in the main manuscript without filtering outliers.

## S9 Analysis without removing outliers

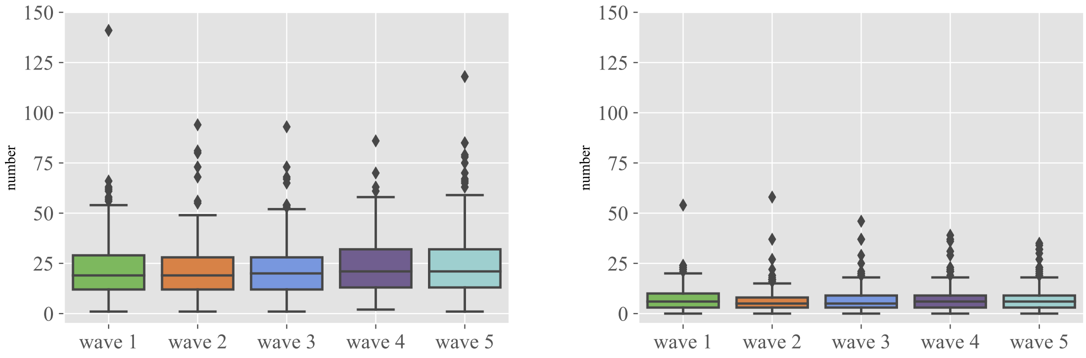


Fig. S24: **The structure of friendships** - Replica of Figure 1 in the main manuscript without filtering outliers.

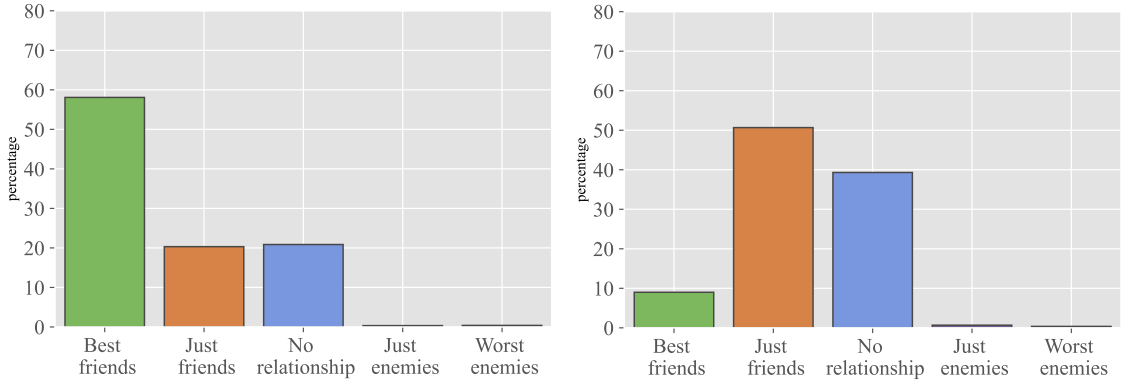


Fig. S25: **The evolution of friendships over time** - Replica of Figure 2 in the main manuscript without filtering outliers.

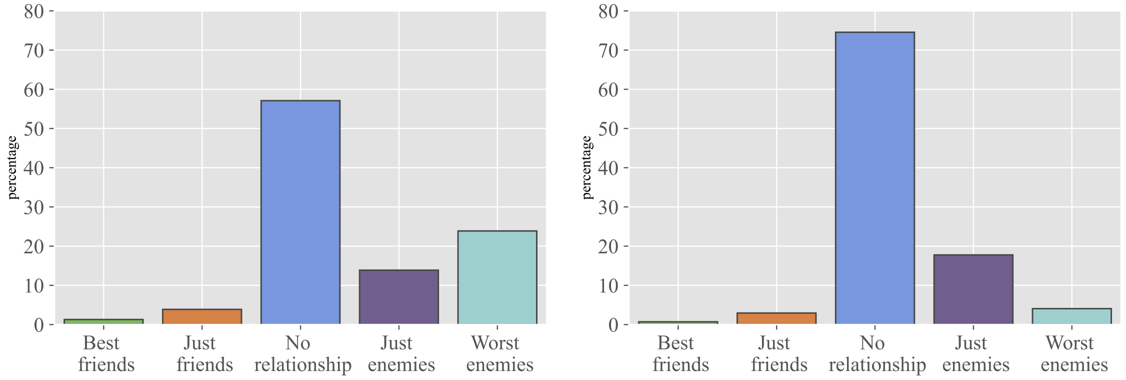


Fig. S26: **The evolution of enmities over time** - Replica of Figure 3 in the main manuscript without filtering outliers.

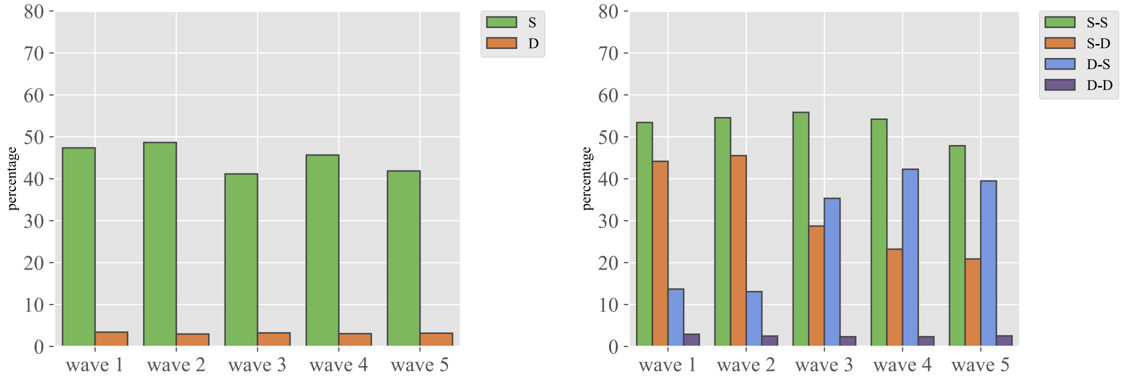


Fig. S27: **The importance of the group for the existence of relationships** - Replica of Figure 4 in the main manuscript without filtering outliers.

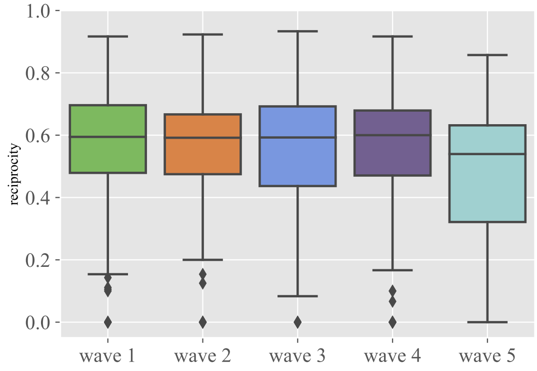


Fig. S28: **The evolution of reciprocity over time -** Replica of Figure 5 in the main manuscript without filtering outliers.

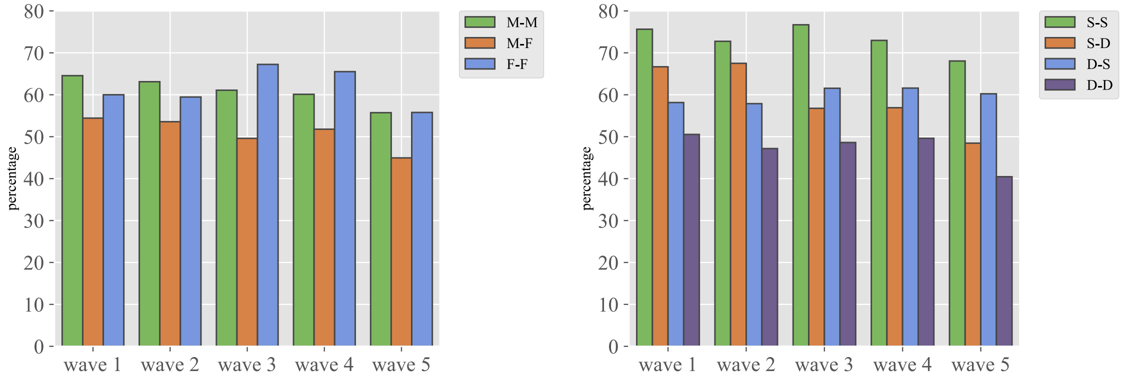


Fig. S29: **The importance of the group for the reciprocity of relationships -** Replica of Figure 6 in the main manuscript without filtering outliers.
